# Supplementary material for: A Large-scale Examination of "Socioeconomic" Fairness in Mobile Networks
Source: arXiv:2304.10190 source file (2023-04-20)
Supplement: Supplementary file 1 [file appendix.tex]

\section{Ethical considerations}
The data collection and retention at network middle-boxes are in accordance with the terms and conditions of the ISP and the local regulations. The terms also include data processing for research and publications as allowed usages of collected data, but do not allow data re-sharing with 3rd parties even for research purposes. Data processing only extracts aggregated information and we do we not have access to any personally identifiable unique identifiers.
